# Supplementary material for: SmartState: Detecting State-Reverting Vulnerabilities in Smart Contracts via Fine-Grained State-Dependency Analysis
Source: arXiv:2406.15988 source file (2024-06-23)
Supplement: Supplementary file 1 [file appendix.tex]

\section{Appendix}
\label{sec:vuln-types}
%We highlight the key characters of the vulnerabilities covered by \system{} as follows.

\begin{figure}[h]
\begin{lstlisting}
contract Barn is Ownable {
  function claimManyFromBarn(tokenIds,unstake) external {
    if (isSheep(tokenIds)){
      owed=_claimSheepFromBarn(tokenIds, unstake);}
    ERC20._mint(msg.sender, owed)
  function _claimSheepFromBarn(tokenId, unstake) internal return (owed){
    unit256 owed= 10000ether
    if (unstake) {
      // 50% chance of all $WOOL stolen, punishment
      if (random(tokenId) & 1 == 1) { 
        _payWolfTax(owed);
        owed = 0;
    else {
      // 20% tax to pay
      _payWolfTax(owed * 20 / 100);  }}
      
contract ERC20 {
  mapping(address => uint256) public _balances;
  function _mint(account, amount) internal {
    _Transfer(address(0), account, amount);}}
    
contract Attacker {
  function FreeofTax(address target, bytes data) public{
    target.call{value:0}(data);
    unit256 After=ERC20.balanceOf(address(this));
    require(After == 10000ether); }
}

\end{lstlisting}

\caption{The details for motivating example illustrated in Figure~\ref{illustrateexample}.}
\label{detailed_example}
%\vspace{-0.1in}
\end{figure}

%\section{Example of false negatives}
